# Supplementary material for: PARIMA: Viewport Adaptive 360-Degree Video Streaming
Source: arXiv:2103.00981 source file (2021-08-20)
Supplement: Supplementary file 1 [file 08.Appendix.tex]

\appendix

\section{Image Projection}

The viewport of a user can be represented as Cartesian coordinates in spherical space. The most common way of representing a $360\degree$ frame is in its `Equirectangular Projection'\cite{equirectangular}. The inter-conversion between the multiple projections are described.
% The projection maps longitudes to constantly spaced vertical lines, and circles of latitude to constantly spaced horizontal lines. In this projection, the objects near the equator are less distorted as compared to the objects near the poles.

\subsection{Spherical to Equirectangular Projection}\label{sp_to_eq}
Cartesian coordinates are mapped to the longitudes and latitudes of a sphere by trivial adjustments of its polar and azimuthal angles.
\par
The convention for the polar and the azimuthal angles that we follow throughout the paper is shown in Figure \ref{fig:spherical_conv}
\begin{figure}[h]
  \centering 
    \includegraphics[width=.3\textwidth]{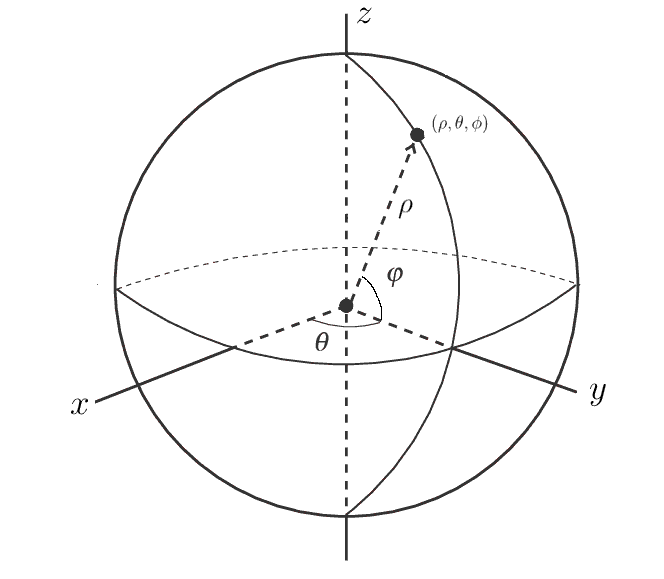}
  \caption{Spherical Coordinates \((\rho, \theta, \phi)\), where $\rho$ is the radial distance, $\phi$ is the polar distance, $\theta$ is the azimuthal angle.}
  \label{fig:spherical_conv}
\end{figure}

Let \((x,y,z)\) be the Cartesian coordinates of a point in sphere. We can represent it in spherical coordinates system \((\rho, \theta, \phi)\) using the following transformation:
\begin{equation}
\begin{split}
\rho  = \sqrt{x^2+y^2+z^2}, \text{   }\theta &= \arctan2{\frac{y}{x}}, \text{   }
\phi = \arcsin{\frac{z}{\rho}}
\end{split}
\end{equation}

 Thus, the longitude\((L_n \in [-180\degree,180\degree])\) and latitude\((L_t) \in [90\degree,90\degree]\) can be computed from $\theta$ and $\phi$ respectively by changing the latter from radian to degree notation
% \begin{equation}\label{long_lat}
% \begin{split}
% L_n  &= \frac{180\degree \theta}{\pi}, \text{  } L_t = \frac{180\degree \phi}{\pi}
% \end{split}
% \end{equation}

The above transformation from \((x,y,z)\) to \((L_n, L_t)\) gives us a representation of a 3-D image in 2-D plane Adjusting $L_n$ and $L_t$ to target image width and height will give the equirectangular position.
\par
For the reverse transformation, an equirectangular image of dimension $(width, height)$ where $width=2*height$ can be projected back into spherical space by considering $\rho = width/2\pi$. $\theta$ and $\phi$ in radians can be calculated from $L_n$ and $L_t$ in degrees by a trivial transformation. For any point $(x_{img}, y_{img})$ in equirectangular frame, we have $L_n$ and $L_t$ as:
\begin{equation}\label{rev_long_lat}
\begin{split}
L_n  &= \frac{x_{img} * 360\degree}{width} - 180\degree, \text{  } L_t = \frac{y_{img} * 180\degree}{height} - 90\degree
\end{split}
\end{equation}

\subsection{Spherical to Cube Map Projection}\label{eq_to_cm}

\par
In cube map projection, a $360\degree$ image is projected onto the sides of a cube and stored as six square textures. We will convert a point in spherical space $(\rho, \theta, \phi)$ to a point in cube map projection.
% Transformation from spherical space to cube map projection can be easily understood using the spherical coordinates $(\rho, \theta, \phi)$ instead of Cartesian coordinates \((x,y,z)\). 
\par
We have $\theta \in [-\pi, \pi]$ and $\phi \in [-\pi/2, \pi/2]$. Thus, the front face of the cube can only capture the pixels of the image having $\theta \in [-\pi/4, \pi/4]$. The projection of a point $(\rho\cos\phi\cos\theta, \rho\cos\phi\sin\theta$, $\rho\sin\phi)$ in spherical domain is $(t\cos\phi\cos\theta, t\cos\phi\sin\theta, t\sin\phi)$ on the plane $x=\rho$ where $t=\frac{\rho}{\cos\phi\cos\theta}$.
\par
Hence the projected point becomes $(\rho, \rho\tan\theta, \rho\tan\phi\sec\theta)$.
\par
Now, if $|\tan\phi\sec\theta| < 1$, then the point will lie on the front face of the cube. Otherwise, it will lie either on the top or the bottom face of the cube, which would then require computing the projection of point $(\rho\cos\phi\cos\theta, \rho\cos\phi\sin\theta, \rho\sin\phi)$ hitting the plane \(z=\rho\) or \(z=-\rho\).
\par
However, it is easy to notice that whenever $\phi>\pi/4$ or $\phi<-\pi/4$, the point will always be projected to the top or bottom face of the cube. Similar will be the arguments for projecting a point on the other faces of the cube.

% \begin{table*}[h]
%     \centering
%     \begin{tabular}{|c|c|c|}
%     \hline
%     \textbf{Face} & \textbf{Coordinates} & \textbf{Conditions} \\ \hline
% Front &  $(\rho, \rho\tan\theta, \rho\tan\phi\sec\theta)$ & $\forall \theta \in [-\pi/4, \pi/4], \phi \in [-\pi/4, \pi/4]$\\ \hline 
% Right & $(\rho\cot\theta, \rho, \rho\tan\phi\cosec\theta)$ & $\forall \theta \in [\pi/4, 3\pi/4], \phi \in [-\pi/4, \pi/4]$ \\ \hline
% Back & $(-\rho, -\rho\tan\theta, -\rho\tan\phi\sec\theta)$ & $\forall \theta \in [3\pi/4, \pi] \cup [-\pi, -3\pi/4], \phi \in [-\pi/4, \pi/4]$ \\ \hline
% Left & $(-\rho\cot\theta, -\rho, -\rho\tan\phi\cosec\theta)$ & $\forall \theta \in [-3\pi/4, -\pi/4], \phi \in [-\pi/4, \pi/4]$ \\ \hline
% Top & $(\rho\cot\phi\cos\theta, \rho\cot\phi\sin\theta, \rho)$ & $\forall \phi>\pi/4$ \\ \hline
% Bottom & $(-\rho\cot\phi\cos\theta, -\rho\cot\phi\sin\theta, -\rho)$ & $\forall \phi<-\pi/4$ \\ \hline
%     \end{tabular}
%     \caption{\textit{Equirectangular to Cube map projection for a point $(\rho\cos\phi\cos\theta, \rho\cos\phi\sin\theta, \rho\sin\phi)$ in spherical space}}
%     \label{eq:cubemap}
% \end{table*}

Thus, for any point $(\rho\cos\phi\cos\theta, \rho\cos\phi\sin\theta, \rho\sin\phi)$, its projected point on any of the face of the cube can be calculated by following the above-mentioned steps.
% is shown in Table \ref{eq:cubemap}.

\par
For inverting a Cube Map Projection of an image of size $(size,size)$ for each face to the Spherical space, consider $\rho=2*size$ and the rest of the steps follow.
